# Supplementary material for: Maintaining Consistency of Data on the Web
Source: arXiv:cs/0501042 source file (2005-02-09)
Supplement: Supplementary file 1 [file appendix.tex]

\onecolumn
\appendix

%{\em Note:} The appendix will be left out in the final version, instead a technical report we are currently working on will be referenced. It is included below for convenience.

%Example~\ref{example:snoop-contexts}--\ref{example:hierarchical-snoop-ct} show the detection of composite events upon the occurrence of primitive event sequences. The sequences reflect the insertions (and modifications in Example~\ref{example:hierarchical-snoop-ct}) of {\sf item} elements ($i_1$, $i_2$) comprising {\sf price} elements ($p_1$, $p_2$), {\sf quantity} elements ($q_1$, $q_{1.1}$, $q_{1.2}$, $q_2$), and {\sf comment} elements ($c_1$). The numerical index of an element represents its hierarchical position, meaning that elements with the same numerical index are hierarchically related, e.g., $p_1$ is a child of $i_1$. In case of two numerical indexes separated by a decimal point, the number before the point represents the element's hierarchical position and the one after the point the time of its insertion, e.g., the insertion of $q_{1.1}$ occurs before the insertion of $q_{1.2}$.

\begin{table}
\caption{Event sequences $S_1 .. S_8$}
\label{table:event-sequences}
\centering
\begin{tabular}[h]{|lll|}
\hline
$S_1 = \{e_{i_1},e_{p_1},e_{q_1},e_{i_2},e_{p_2},e_{q_2}\}$ &&
$S_6 = \{e_{i_1},e_{p_1},e_{c_1},e_{q_1},e_{i_2}\}$ \\ 
$S_2 = \{e_{i_1},e_{i_2},e_{p_1},e_{p_2},e_{q_1},e_{q_2}\}$ &&
$S_7 = \{e_{i_1},e_{p_1},e_{q_{1.1}},e_{c_1},e_{q_{1.2}},e_{i_2}\}$ \\ 
$S_3 = \{e_{i_1},e_{i_2},e_{p_1},e_{q_1},e_{p_2},e_{q_2}\}$ &&
$S_8 = \{e_{i_1},e_{p_1},e_{i_2},e_{p_2},e_{q_1},e_{q_2}\}$ \\
$S_4 = \{e_{i_1},e_{i_2},e_{p_1},e_{q_2},e_{p_2},e_{q_1}\}$ &&
$S_9 = \{e_{q_{1.1}},e_{q_2},e_{q_{1.2}},e_{p_2},e_{p_1}\}$ \\
$S_5 = \{e_{i_1},e_{p_1},e_{q_1},e_{i_2}\}$ && \\
\hline
\end{tabular}
\end{table}

\begin{example}
\label{example:snoop-contexts}
%Table~\ref{tab:adapted-evt-graphs} shows raised composite events within the event tree depicted in Figure~\ref{fig:evtgraph-pt-derivation} when employing the refined event algebra introduced in Section~\ref{section:adaption} with {\em contexts from Snoop}. Only composite events raised by the root of the tree are shown by their constituent events, e.g., $\{e_{i_1}e_{p_1}e_{q_1}\}^c$. The table's rationale is twofold: first, to exemplify that incorrect composite events are raised when any of Snoop's contexts is used (for which one falsificating event sequence would suffice), and second, to introduce the unfamiliar reader to Snoop's contexts.The table does not show the unrestricted context which basically forms the cartesian product of all events. Naturally, it raises even more incorrect composite events.
\end{example}

%\begin{tabbing}
%\quad \=\quad \=\quad \=\quad \=\quad \=\quad \=\quad \=\quad \kill
%{\em Event types:} \\
%$et_i:=\langle {\sf ins}, {\sf/order/item}\rangle$, \\
%$et_p:=\langle {\sf ins}, {\sf/order/item/price}\rangle$, \\
%$et_q:=\langle {\sf ins}, {\sf/order/item/quantity}\rangle$ \\
%{\em Events:} \\
%$e_{i_1}:=\langle et_i, /o_1/i_1 \rangle$, $e_{i_2}:=\langle et_i, /o_2/i_2 \rangle$, \\
%$e_{p_1}:=\langle et_p, /o_1/i_1/p_1 \rangle$, $e_{p_2}:=\langle et_p, /o_2/i_2/p_2 \rangle$, \\
%$e_{p_1}:=\langle et_q, /o_1/i_1/q_1 \rangle$, $e_{q_2}:=\langle et_q, /o_2/i_2/q_2 \rangle$ \\
%{\em Event Sequences:} \\
%1: $e_{i_1}e_{p_1}e_{q_1}e_{i_2}e_{p_2}e_{q_2}$, 
%2: $e_{i_1}e_{i_2}e_{p_1}e_{p_2}e_{q_1}e_{q_2}$, \\
%3: $e_{i_1}e_{i_2}e_{p_1}e_{q_1}e_{p_2}e_{q_2}$,
%4: $e_{i_1}e_{i_2}e_{p_1}e_{q_2}e_{p_2}e_{q_1}$.
%\end{tabbing}

\begin{sidewaystable}
\centering

\caption{Raised Composite Events when using Contexts from Snoop}
\label{tab:adapted-evt-graphs}

\begin{tabular}[h]{|c|c|c|c|c|c|c|}
\hline
- & $t_1$ & $t_2$ & $t_3$ & $t_4$ & $t_5$ & $t_6$ \\
\hline \hline
\multicolumn{7}{|c|}{Cumulative Context} \\ \hline
$S_1$ & $e_{i_1}$ & $e_{p_1}$ & $e_{q_1}, \{e_{i_1} e_{p_1} e_{q_1}\}^c$ & $e_{i_2}$ & $e_{p_2}$ & $e_{q_2}, \{e_{i_2} e_{p_2} e_{q_2}\}^c$ \\ \hline
$S_2$ & $e_{i_1}$ & $e_{i_2}$ & $e_{p_1}$ & $e_{p_2}$ & $e_{q_1}, \{e_{i_1} e_{i_2} e_{p_1} e_{p_2} e_{q_1}\}^c$ & $e_{q_2}$ \\ \hline
$S_3$ & $e_{i_1}$ & $e_{i_2}$ & $e_{p_1}$ & $e_{q_1}, \{e_{i_1} e_{i_2} e_{p_1} e_{q_1}\}^c$ & $e_{p_2}$ & $e_{q_2}, (\{e_{p_2} e_{q_2}\}^c)$ \\ \hline
$S_4$ & $e_{i_1}$ & $e_{i_2}$ & $e_{p_1}$ & $e_{q_2}, \{e_{i_1} e_{i_2} e_{p_1} e_{q_2}\}^c$ & $e_{p_2}$ & $e_{q_1}, (\{e_{p_2} e_{q_1}\}^c)$ \\
\hline \hline
\multicolumn{7}{|c|}{Chronicle Context} \\ \hline
$S_1$ & $e_{i_1}$ & $e_{p_1}$ & $e_{q_1}, \{e_{i_1} e_{p_1} e_{q_1}\}^c$ & $e_{i_2}$ & $e_{p_2}$ & $e_{q_2}, \{e_{i_2} e_{p_2} e_{q_2}\}^c$ \\ \hline
$S_2$ & $e_{i_1}$ & $e_{i_2}$ & $e_{p_1}$ & $e_{p_2}$ & $e_{q_1}, \{e_{i_1} e_{p_1} e_{q_1}\}^c$ & $e_{q_2}, \{e_{i_2} e_{p_2} e_{q_2}\}^c$ \\ \hline
$S_3$ & $e_{i_1}$ & $e_{i_2}$ & $e_{p_1}$ & $e_{q_1}, \{e_{i_1} e_{p_1} e_{q_1}\}^c$ & $e_{p_2}$ & $e_{q_2}, \{e_{i_2} e_{p_2} e_{q_2}\}^c$ \\ \hline
$S_4$ & $e_{i_1}$ & $e_{i_2}$ & $e_{p_1}$ & $e_{q_2}, \{e_{i_1} e_{p_1} e_{q_2}\}^c$ & $e_{p_2}$ & $e_{q_1}, \{e_{i_2} e_{p_2} e_{q_1}\}^c$ \\ 
\hline \hline
\multicolumn{7}{|c|}{Recent Context} \\ \hline
$S_1$ & $e_{i_1}$ & $e_{p_1}$ & $e_{q_1}, \{e_{i_1} e_{p_1} e_{q_1}\}^c$ & $e_{i_2}$ & $e_{p_2}, \{e_{i_2} e_{p_2} e_{q_1}\}^c$ & $e_{q_2}, \{e_{i_2} e_{p_2} e_{q_2}\}^c$ \\ \hline
$S_2$ & $e_{i_1}$ & $e_{i_2}$ & $e_{p_1}$ & $e_{p_2}$ & $e_{q_1}, \{e_{i_2} e_{p_2} e_{q_1}\}^c$ & $e_{q_2}, \{e_{i_2} e_{p_2} e_{q_2}\}^c$ \\ \hline
$S_3$ & $e_{i_1}$ & $e_{i_2}$ & $e_{p_1}$ & $e_{q_1}, \{e_{i_2} e_{p_1} e_{q_1}\}^c$ & $e_{p_2}, \{e_{i_2} e_{p_2} e_{q_1}\}^c$ & $e_{q_2}, \{e_{i_2} e_{p_2} e_{q_2}\}^c$ \\ \hline
$S_4$ & $e_{i_1}$ & $e_{i_2}$ & $e_{p_1}$ & $e_{q_2}, \{e_{i_2} e_{p_1} e_{q_2}\}^c$ & $e_{p_2}, \{e_{i_2} e_{p_2} e_{q_2}\}^c$ & $e_{q_1}, \{e_{i_2} e_{p_2} e_{q_1}\}^c$ \\

\hline \hline
\multicolumn{7}{|c|}{Continuous Context} \\ \hline
$S_1$ & $e_{i_1}$ & $e_{p_1}$ & $e_{q_1}, \{e_{i_1}e_{p_1}e_{q_1}\}^c$ & $e_{i_2}$ & $e_{p_2}, \{e_{i_2}e_{p_2}e_{q_1}\}^c$ & $e_{q_2}, (\{e_{p_2}e_{q_2}\}^c)$ \\ \hline
$S_2$ & $e_{i_1}$ & $e_{i_2}$ & $e_{p_1}$ & $e_{p_2}$ & $e_{q_1},\dag_1$ & $e_{q_2}$ \\ \hline
$S_3$ & $e_{i_1}$ & $e_{i_2}$ & $e_{p_1}$ & $e_{q_1},\dag_2$ & $e_{p_2}, (\{e_{p_2}e_{q_1}\}^c)$ & $e_{q_2}, (\{e_{p_2}e_{q_2}\}^c)$ \\ \hline
$S_4$ & $e_{i_1}$ & $e_{i_2}$ & $e_{p_1}$ & $e_{q_2},\dag_3$ & $e_{p_2}, (\{e_{p_2}e_{q_2}\}^c)$ & $e_{q_1}, (\{e_{p_2}e_{q_1}\}^c)$ \\ 
\hline
\multicolumn{7}{|c|}{
    $\dag_1$: $\{e_{i_1}e_{p_1}e_{q_1}\}^c, \{e_{i_1}e_{p_2}e_{q_1}\}^c, 
    \{e_{i_2}e_{p_1}e_{q_1}\}^c, \{e_{i_2}e_{p_2}e_{q_1}\}^c$
    $\dag_2$: $\{e_{i_1}e_{p_1}e_{q_1}\}^c, \{e_{i_2}e_{p_1}e_{q_1}\}^c$
    $\dag_3$: $\{e_{i_1}e_{p_1}e_{q_2}\}^c, \{e_{i_2}e_{p_1}e_{q_2}\}^c$
}
\\ \hline
\end{tabular}
\end{sidewaystable} 

\begin{example}
Table~\ref{tab:hierarchical-context} shows raised composite events within the event tree depicted in Figure~\ref{fig:evtgraph-pt-derivation} when employing the refined event algebra and the \textit{hierarchical context} introduced in Section~\ref{section:extension}. 
Only composite events raised by the root of the tree are shown by their constituent events.
All raised events are correct, i.e., their constituent events are hierarchically related. 
The same composite events are raised independent of the context from Snoop that is combined with the hierarchical context.
\end{example}

\begin{table}
\caption{Raised composite events when using the hierarchical context introduced in Section~\ref{section:extension}}
\label{tab:hierarchical-context}

\centering
\begin{tabular}[h]{|c|c|c|c|c|c|c|}
\hline
- & $t_1$ & $t_2$ & $t_3$ & $t_4$ & $t_5$ & $t_6$  \\
\hline \hline
\multicolumn{7}{|c|}{Hierarchical Context} \\ \hline
$S_1$ & $e_{i_1}$ & $e_{p_1}$ & $e_{q_1}, \{e_{i_1}e_{p_1}e_{q_1}\}^c$ & $e_{i_2}$ & $e_{p_2}$ & $e_{q_2}, \{e_{i_2}e_{p_2}e_{q_2}\}^c$ \\ \hline
$S_2$ & $e_{i_1}$ & $e_{i_2}$ & $e_{p_1}$ & $e_{p_2}$ & $e_{q_1}, \{e_{i_1}e_{p_1}e_{q_1}\}^c$ & $e_{q_2}, \{e_{i_2}e_{p_2}e_{q_2}\}^c$ \\ \hline
$S_3$ & $e_{i_1}$ & $e_{i_2}$ & $e_{p_1}$ & $e_{q_1}, \{e_{i_1}e_{p_1}e_{q_1}\}^c$ & $e_{p_2}$ & $e_{q_2}, \{e_{i_2}e_{p_2}e_{q_2}\}^c$ \\ \hline
$S_4$ & $e_{i_1}$ & $e_{i_2}$ & $e_{p_1}$ & $e_{q_2}$ & $e_{p_2}, \{e_{i_2}e_{p_2}e_{q_2}\}^c$ & $e_{q_1}, \{e_{i_1}e_{p_1}e_{q_1}\}^c$ \\
\hline
\end{tabular}
\end{table} 

\begin{example}
Table~\ref{tab:termination-modes} shows raised composite events within the event tree depicted in Figure~\ref{fig:evtgraph.mult-op} when different \textit{termination modes} and the hierarchical context are used. Raised composite events are represented by symbol $e^c$ with the alphabetical index indicating its event type and the numerical index indicating its hierarchical position. %, e.g., $e^c_{q_1}$ is an event of type $E^c_q$ in position $1$.
Again, independent of the context from Snoop that is combined with the hierarchical context the same composite events are raised.
\end{example}

\begin{sidewaystable}
\centering

\caption{Raised Composite Events in Hierarchical Context when different Termination Modes are used}
\label{tab:termination-modes}

\begin{tabular}[h]{|c|c|c|c|c|c|c|}
\hline
- & $t_1$ & $t_2$ & $t_3$ & $t_4$ & $t_5$ & $t_6$ \\
\hline \hline
% ########################################
% #
% ########################################
\multicolumn{7}{|c|}{(1a) $\bigtriangleup: {\sf earliest}, \times[1,\infty]: {\sf earliest}$} \\
\hline
$S_6$ & $e_{i_1},e^c_{c_{1}}$ & $e_{p_1}$ & $e_{q_1}, e^c_{q_1},e^c_{h_1}, {\bf e^c_{i_1}}$ & $e_{i_2},e^c_{c_2}$ & -- & -- \\
\hline
$S_7$ & $e_{i_1},e^c_{c_{1.1}}$ & $e_{p_1}$ & $e_{c_1}, e^c_{c_{1.2}}$ & $e_{q_1}, e^c_{q_1}, e^c_{h_1}, {\bf e^c_{i_1}}$ & $e_{i_2},e^c_{c_2}$ & -- \\
\hline
$S_8$ & $e_{i_1},e^c_{c_{1.1}}$ & $e_{p_1}$ & $e_{q_{1.1}}, e^c_{q_{1.1}}, e^c_{h_1}, {\bf e^c_{i_1}}$ & $e_{c_1}, e^c_{c_{1.2}}$ & $e_{q_{1.2}}, e^c_{q_{1.2}}$ & $e_{i_2},e^c_{c_2}$ \\
\hline
$S_9$ & $e_{i_1},e^c_{c_{1}}$ & $e_{p_1}$ & $e_{i_2},e^c_{c_2}$ & $e_{p_2}$ & $e_{q_1},e^c_{q_1},e^c_{h_1}, {\bf e^c_{i_1}}$ & $e_{q_2},e^c_{q_2},e^c_{h_2}, {\bf e^c_{i_2}}$ \\
\hline \hline
% ########################################
% #
% ########################################
\multicolumn{7}{|c|}{(1b) $\bigtriangleup: {\sf earliest}, \times[1,\infty]: {\sf non}$-${\sf local}$} \\
\hline
$S_6$ & $e_{i_1},e^c_{c_1}$ & $e_{p_1}$ & $e_{q_1}$ & $e_{i_2},e^c_{c_2}, e^c_{q_1}, e^c_{h_1}, {\bf e^c_{i_1}}$ & -- & -- \\
\hline
$S_7$ & $e_{i_1},e^c_{c_{1.1}}$ & $e_{p_1}$ & $e_{c_1},e^c_{c_{1.2}}$ & $e_{q_1}$ & $e_{i_2},e^c_{c_2}, e^c_{q_1}, e^c_{h_1}, {\bf e^c_{i_1}}$ & -- \\
\hline
$S_8$ & $e_{i_1},e^c_{c_{1.1}}$ & $e_{p_1}$ & $e_{q_{1.1}}$ & $e_{c_1}, e^c_{c_{1.2}}$ & $e_{q_{1.2}}$ & $e_{i_2},e^c_{c_2},e^c_{q_1},e^c_{h_1},{\bf e^c_{i_1}}$ \\
\hline
$S_9$ & $e_{i_1},e^c_{c_1}$ & $e_{p_1}$ & $e_{i_2},e^c_{c_2}$ & $e_{p_2}$ & $e_{q_1}$ & $e_{q_2}, e^c_{q_1}, e^c_{h_1}, {\bf e^c_{i_1}}$ \\
\hline \hline
% ########################################
% #
% ########################################
\multicolumn{7}{|c|}{(2a) $\bigtriangleup: {\sf non}$-${\sf local}, \times[1,\infty]: {\sf earliest}$} \\
\hline
$S_6$ & $e_{i_1},e^c_{c_1}$ & $e_{p_1}$ & $e_{q_1}, e^c_{q_1}$ & $e_{i_2},e^c_{c_2}, e^c_{h_1}, {\bf e^c_{i_1}}$ & -- & -- \\
\hline
$S_7$ & $e_{i_1},e^c_{c_{1.1}}$ & $e_{p_1}$ & $e_{c_1},e^c_{c_{1.2}}$ & $e_{q_1}, e^c_{q_1}$ & $e_{i_2},e^c_{c_2}, e^c_{h_1}, {\bf e^c_{i_1}}$ & --\\
\hline
$S_8$ & $e_{i_1},e^c_{c_{1.1}}$ & $e_{p_1}$ & $e_{q_{1.1}}, e^c_{q_{1.1}}$ & $e_{c_1}, e^c_{c_{1.2}}$ & $e_{q_{1.2}}, e^c_{q_{1.2}}$ & $e_{i_2},e^c_{c_2}, e^c_{h_1}, {\bf e^c_{i_1}}$ \\
\hline
$S_9$ & $e_{i_1},e^c_{c_1}$ & $e_{p_1}$ & $e_{i_2},e^c_{c_2}$ & $e_{p_2}$ & $e_{q_1}, e^c_{q_1}$ & $e_{q_2},e^c_{h_1},{\bf e^c_{i_1}}$ \\
\hline \hline
% ########################################
% #
% ########################################
\multicolumn{7}{|c|}{(2b) $\bigtriangleup: {\sf non}$-${\sf local}, \times[1,\infty]: {\sf non}$-${\sf local}$} \\
\hline
$S_6$ & $e_{i_1},e^c_{c_1}$ & $e_{p_1}$ & $e_{q_1}$ & $e_{i_2},e^c_{c_2}, e^c_{q_1}, e^c_{h_1}, {\bf e^c_{i_1}}$ & -- & -- \\
\hline
$S_7$ & $e_{i_1},e^c_{c_{1.1}}$ & $e_{p_1}$ & $e_{c_1}, e^c_{c_{1.2}}$ & $e_{q_1}$ & $e_{i_2},e^c_{c_2}, e^c_{q_1}, e^c_{h_1}, {\bf e^c_{i_1}}$ & -- \\
\hline
$S_8$ & $e_{i_1},e^c_{c_{1.1}}$ & $e_{p_1}$ & $e_{q_{1.1}}$ & $e_{c_1}, e^c_{c_{1.2}}$ & $e_{q_{1.2}}$ & $e_{i_2},e^c_{c_2}, e^c_{q_1}, e^c_{h_1}, {\bf e^c_{i_1}}$ \\
\hline
$S_9$ & $e_{i_1},e^c_{c_1}$ & $e_{p_1}$ & $e_{i_2},e^c_{c_2}$ & $e_{p_2}$ & $e_{q_1}$ & $e_{q_2}, e^c_{q_1}, e^c_{h_1}, {\bf e^c_{i_1}}$ \\
\hline
\end{tabular} 
\end{sidewaystable} 

% As noted in Section~\ref{section:hierarchical-context} each of the contexts of Snoop can be combined with the hierarchical context, since selection by hierarchy and time are orthogonal. Example~\ref{example:hierarchical-snoop-ct} shows how every combination of the hierarchical context with contexts from Snoop raises composite events.

\begin{example}
\label{example:hierarchical-snoop-ct}
Event expression {\sf $*$(item/quant) $\bigtriangleup$ upd(item/price)} is used to detect when both price and quantity information of an order item are modified. Table~\ref{tab:hierarchical-snoop-contexts} shows raised composite events (represented by their constituent events) for the above expression in the \textit{hierarchical variants of Snoop's contexts}. Events that remain in the event graph after $t_5$ are shown in the rightmost column for completeness.
\end{example}

\begin{sidewaystable}
\centering
\caption{Combination of the Hierarchical Context with Contexts from Snoop}
\label{tab:hierarchical-snoop-contexts}

\begin{tabular}[h]{|c|c|c|c|c|c|l|}
\hline
- & $t_1$ & $t_2$ & $t_3$ & $t_4$ & $t_5$ & unconsumed events\\
\hline \hline
\multicolumn{7}{|c|}{Hierarchical Cumulative Context} \\ \hline
$S_5$ & $e_{q_{1.1}}$ & $e_{q_2}$ & $e_{q_{1.2}}$ & $e_{p_2}, \{e_{p_2} e_{q_2}\}^c$ & $e_{p_1}, \{e_{p_1} e_{q_{1.1}} e_{q_{1.2}}\}^c$ & -- \\
\hline \hline

\multicolumn{7}{|c|}{Hierarchical Chronicle Context} \\ \hline
$S_5$ & $e_{q_{1.1}}$ & $e_{q_2}$ & $e_{q_{1.2}}$ & $e_{p_2}, \{e_{p_2} e_{q_2}\}^c$ & $e_{p_1}, \{e_{p_1} e_{q_{1.1}}\}^c$ & $e_{q_{1.2}}$ \\
\hline \hline

\multicolumn{7}{|c|}{Hierarchical Recent Context} \\ \hline
$S_5$ & $e_{q_{1.1}}$ & $e_{q_2}$ & $e_{q_{1.2}}$ & $e_{p_2}, \{e_{p_2} e_{q_2}\}^c$ & $e_{p_1}, \{e_{p_1} e_{q_{1.2}}\}^c$ & $e_{p_1}, e_{q_{1.2}}, e_{p_2}, e_{q_2}$ \\
\hline \hline

\multicolumn{7}{|c|}{Hierarchical Continuous Context} \\ \hline
$S_5$ & $e_{q_{1.1}}$ & $e_{q_2}$ & $e_{q_{1.2}}$ & $e_{p_2}, \{e_{p_2} e_{q_2}\}^c$ & $e_{p_1}, \{e_{p_1} e_{q_{1.1}}\}^c, \{e_{p_1} e_{q_{1.2}}\}^c$ & $e_{p_1}, e_{p_2}$\\
\hline
\end{tabular}
\end{sidewaystable}
