# Supplementary material for: Maintaining Consistency of Data on the Web
Source: arXiv:cs/0501042 source file (2005-02-09)
Supplement: Supplementary file 3 [file smwp_appendix.tex]

% In Kommentar gesetzte Stellen kennzeichnen diejenige EBNF, die den Prototypen im Gegensatz
% bum alter ADC Paper auszeichnet.
\section{SMWP}
\subsection*{Schema Definition Language}
\label{AppendixSDL}

This section contains a complete specification of the schema definition language as introduced in Section~\ref{SchemaDefinitionLanguage}. Terms ``/*'' and ``*/'' are used to delimit comments.

\begin{tabbing}
\quad \=\quad \=\quad \=\quad \=\quad \=\quad \=\quad \=\quad \=\quad \kill
{\em SMWPStmt} := (CreateStmt $|$ DropStmt $|$ ShowStmt $|$ AlterStmt) ``;''. \\
\\
{\it /* Create Statement */} \\
{\em CreateStmt} := \\
\>\>``CREATE'' (FCCreateStmt $|$ PCCreateStmt $|$ ParamCreateStmt). \\
%FCCreateStmt  = PFCCreateStmt $|$ DFCCreateStmt $|$ AFCCreateStmt. \\
{\em FCCreateStmt} : = PFCCreateStmt $|$ DFCCreateStmt. \\
{\em PFCCreateStmt} :=  \\
\>\>``PRIMARY FRAGMENT CLASS'' FCSignature \\
\>\>``FRAGMENTATION BASE CLASS'' FCSignature \\
\>\>[``TUPLE SELECTION PREDICATE'' SQLExpr] \\
\>\>[``FRAGMENT SELECTION PREDICATE'' SQLExpr]. \\
%\>[ XMLPublishFCStmt ]. \\
{\em DFCCreateStmt} :=  \\
\>\>``DERIVED FRAGMENT CLASS'' FCSignature \\
\>\>``FRAGMENTATION BASE CLASS'' FCSignature [``AS'' Ident] \\
\>\>``DERIVATION BASE CLASS'' FCSignature [``AS'' Ident] \\
\>\>``JOIN BY'' SQLExpr. \\
%\>[ XMLPublishFCStmt ]. \\
\\
{\em PCCreateStmt} :=  \\
\>\>``PAGE CLASS'' PCSignature \\
\>\>[``FILENAME'' FileName] \\
%\>\>[''GENERATION APPROACH'' (''coreSMWP'' $|$ ''pullOfFragments'' $|$ ''onTheFly'')] \\
\>\>``FOUNDATION FRAGMENT CLASS'' PCFCMapping \\
\>\>\{``FRAGMENT CLASS'' PCFCMapping\}. \\
%\>[ XMLPublishPCStmt ]. \\
{\em PCFCMapping} := FCSignature [``AS'' Ident] \\
\>\>[ParameterMap] \{InternalPageRef $|$ ExternalPageRef\}. \\
{\em ParameterMap} := \\
\>\>``PARAMETER MAP'' Ident ``AS'' Ident \{``,'' Ident ``AS'' Ident\}. \\
{\em InternalPageRef} := \\
\>\>``INTERNAL LINK TO FRAGMENT CLASS'' FCSignature \\
\>\>[``AS'' Ident] ``JOIN BY'' SQLExpr. \\
{\em ExternalPageRef} := \\
\>\>``EXTERNAL LINK TO PAGE CLASS'' PCSignature [``AS'' Ident] \\
\>\>``CONTAINING FRAGMENT CLASS'' FCSignature [``AS'' Ident] \\
\>\>``JOIN BY'' SQLExpr. \\
\\
{\em ParamCreateStmt} := VBPCreateStmt $|$ PBPCreateStmt. \\
{\em VBPCreateStmt} := \\
\>\>``VALUE BASED PARAMETER'' Ident ``ON'' FCSignature \\
\>\>(UseReferenceRelationStmt $|$ CreateReferenceRelationStmt). \\
{\em UseReferenceRelationStmt} := \\
\>\>``USE REFERENCE RELATION'' Ident ``('' Ident ``)''. \\
{\em CreateReferenceRelationStmt} := ``CREATE REFERENCE RELATION''. \\ % SYNC-POLICY'' (''expansive'' $|$ ''synchronized''). \\
{\em PBPCreateStmt} := \\
\>\>``PREDICATE BASED PARAMETER'' Ident ``ON'' FCSignature \\
\>\>``PREDICATES \{'' ``(``'' Ident ``'','' SQLExpr ``)'' \\
\>\>\{``,'' ``(``'' Ident ``'','' SQLExpr ``)''\} ``\}''. \\
%XMLPublishFCStmt = \\
%\>''PUBLISH FRAGMENT AS NAME'' ElementName \\
%\>''AND TUPLE AS NAME'' ElementName ''IN NAMESPACE'' Namespace. \\
\\
{\em SQLExpr} := ``\{'' \{ANY\} ``\}''. \\
%XMLPublishPCStmt = ''PUBLISH PAGE AS NAME'' ElementName ''IN NAMESPACE'' Namespace. \\
\\
{\it /* Drop Statement */} \\
{\em DropStmt} := ``DROP'' (FCDropStmt $|$ PCDropStmt $|$ ParamDropStmt). \\
{\em FCDropStmt} := ``FRAGMENT CLASS'' FCSignature. \\
{\em PCDropStmt} := ``PAGE CLASS'' PCSignature. \\
{\em ParamDropStmt} := ``PARAMETER'' Ident ``DEFINED UPON'' FCSignature. \\

\\
{\it /* Show Statement */} \\
{\em ShowStmt} := ``SHOW'' (FCShowStmt $|$ PCShowStmt $|$ ParamShowStmt). \\
{\em FCShowStmt} := ``FRAGMENT CLASS'' (FCSignature $|$ ``*''). \\
{\em PCShowStmt} := ``PAGE CLASS'' (PCSignature $|$ ``*''). \\
{\em ParamShowStmt} := ``PARAMETER'' (Ident $|$ ``*'') \\
\>\>[``DEFINED UPON'' FCSignature]. \\

\\
{\it /* Alter Statement */} \\
{\em AlterStmt} := ``ALTER'' PCAlterStmt. \\
%AlterStmt = ''ALTER'' (FCAlterStmt $|$ PCAlterStmt). \\
%FCAlterStmt = ''FRAGMENT CLASS'' ClassName (''TO'' XMLPublishFCStmt $|$ ''CLEAR PUBLICATION SPECIFICATION''). \\
{\em PCAlterStmt} := \\
\>\>``PAGE CLASS'' PCSignature (PCAlterAddStmt $|$ PCAlterDropStmt). \\
{\em PCAlterAddStmt} := \\
\>\>[PCAlterAliasStmt] ``ADD FRAGMENT CLASS'' PCFCMapping. \\
{\em PCAlterAliasStmt} := \\
\>\>``REFERRING TO FRAGMENT CLASS'' \\
\>\>FCSignature ``AS'' Ident \{``,'' FCSignature ``AS'' Ident\}. \\
{\em PCAlterDropStmt} := ``DROP FRAGMENT CLASS'' FCSignature. \\

\\
{\it /* Miscellaneous */} \\
{\it /* Signature of a fragment class */} \\
{\em FCSignature} := FCName ``$<$'' [ParamName \{``,'' ParamName\}] ``$>$''. \\
{\it /* Signature of a page class */} \\
{\em PCSignature} := PCName ``$<$'' [ParamName \{``,'' ParamName\}] ``$>$''. \\
{\em ParamName} := Ident. {\it /* Name of a parameter */} \\
{\em FCName} := Ident. {\it /* Name of a fragment class */} \\
{\em PCName} := Ident. {\it /* Name of a page class */} \\
{\em FileName} := Ident ``.'' Ident. {\it /* Filename-Template for pages */}  \\
%ElementName = cf. XML Specification
%Namespace = cf. URI/XML Namespace Specification
{\em Ident} := letter \{letter $|$ digit $|$ ``\_'' $|$ ``-''\}. \\
{\em letter} := ``A$|$B$|$..$|$Z$|$a$|$b$|$..$|$z''. \\
{\em digit} := ``0$|$1$|$..$|$9''. \\
\end{tabbing}

% ~~~~~~~~~~~~~~~~~~~~~~~~~~~~~~~~~~~~~~~~~~~~~~~~~~~~~~~~~~~~
%
% TABLE
%
% ~~~~~~~~~~~~~~~~~~~~~~~~~~~~~~~~~~~~~~~~~~~~~~~~~~~~~~~~~~~~

\subsection*{Naming Conventions}

%Abbreviations are used to refer to artifacts of the SMWP approach such as fragment classes and content relations throughout the paper from within text and algorithms. In general, 
When referring to artifacts of the SMWP approach such as fragment classes and content relations, placeholders and variables are written in italics (e.g., {\it F$<$L$>$} or {\it FC\_F\_L}) while concrete artifacts are denoted in sans-serif (e.g., {\sf Prem\-Wines$<$region$>$} or {\sf FC\_Prem\-Wines\_region}). 
%The definitions in EBNF below summarize how acronyms are formed. They partly make use definitions from Appendix~\ref{AppendixSDL}.

Artifacts of the realization model (i.e., relations and triggers) are named using prefixes to explicitly distinguish their kind. Table~\ref{table:prefixes} describes the prefixes used.
% Relations are named containing the respective fragment class' name and parameters, following the form ``{\it prefix} `{\sf \_}' {\it name} `{\sf \_}' {\it parameters}". Every trigger is named after the form ``{\it prefix} `{\sf \_}' {\it source-relation} `{\sf -To-}' {\it target-relation}", where it propagates modifications on the source-relation to the target-relation.

\begin{table}
\setcounter{section}{10}
\caption{Prefixes used in Naming SMWP Artifacts}
\label{table:prefixes}
\begin{tabular}[h]{|c|p{12cm}|}
\hline
Prefix & Description \\
\hline \hline
FC & {\em Content relation} storing a fragment class' data, e.g., {\sf FC\_\-Prem\-Wines\_\-re\-gion} stores data of fragment class {\sf Prem\-Wines$<$re\-gion$>$}. \\
FR & {\em Fragmentation relation} storing fragmentation, e.g., {\sf FR\_\-Prem\-Wines\_\-re\-gion} stores fragmentation of fragment class {\sf Prem\-Wines$<$re\-gion$>$}. \\
RV & {\em Reference relation} storing a parameter's domain, e.g., {\sf RV\_\-Win\-eries\_\-re\-gion} stores the domain of parameter {\sf region} defined on root fragment class {\sf Wineries$<$$>$}. \\ \hline \hline
AT & {\em Auxiliary trigger} used in propagating modifications of a derivation base class' content relation to a derived fragment class' content relation. 
 \\
%, e.g., {\sf AT\_FC\_PremWineries\_region-To-FC\_Prem\-Wines\_region} \\ 
%, e.g., {\sf AT\_Deriv\-Base\-To\-Derived\-FC-FC\_Prem\-Wines\_region} \\
%
CT & {\em Content trigger} propagating modifications between content relations. \\ 
%, e.g., {\sf CT\_Frag\-Base\-To\-Primary\-FC-FC\_PremWineries\_region} propagates modifications to {\sf FC\_Prem\-Win\-eries\_region} \\
%
FT & {\em Fragmentation trigger} propagating modifications between fragmentation relations and from reference relations to fragmentation relations. \\ %, e.g., {\sf FT\_Frag\-Base\-Regions-ToPrimaryFC\-FR\_PremWineries\_region} propagates modifications to {\sf FR\_PremWineries\_region} \\
ST & {\em Serialization trigger} propagating modifications of data and fragmentation to pages. \\
\hline
\end{tabular}
\end{table}
